# Supplementary material for: Tools in the Loop: Quantifying Uncertainty of LLM Question Answering Systems That Use Tools
Source: arXiv:2505.16113 source file (2025-05-22)
Supplement: Supplementary file 1 [file appendix.tex]

\section*{Appendix}
\subsection*{Additional Experiment details}

We use the all-MiniLm-L6-v2 model from Sentence Embeddings \cite{reimers-2019-sentence-bert} to encode the input sequences into vectors. Then, we use  a simple MLP with 1 hidden layer of 64 hidden units for the posterior models. In the case of $H(z|a,y)$, we predict logits over the space of $z$ and optimize using cross entropy. In the case of $H(a|x,y)$, we treat each feature as independant given the input and fit a normal distribution (i.e. a mean and a variance), conditioned on the vector embeddings of $x$ and $y$.

For the RAG system, we use the 'msmarco-distilbert-base-v2' model from Sentence Embeddings to compute vector embeddings of documents and queries.
